# Supplementary material for: MAP's not dead yet: Uncovering true language model modes by conditioning away degeneracy
Source: arXiv:2311.08817 source file (2024-08-08)
Supplement: Supplementary file 1 [file cond_beam_search_algorithm.tex]

\algnewcommand{\LineComment}[1]{\State \(\triangleright\) #1}
\begin{algorithm}
\caption{Conditional beam search. This searches for an output with a sequence $x$ with a high value of $\pmodel(x, A(x) = a)$ for some target attribute $a$. In order to execute this efficiently one needs to efficiently compute $\pmodel$ and $\pclf$ to avoid recomputation. This will typically involve caching transformer hidden states, as is standard for causal transformers.}\label{alg:beam_cond}
 \hspace*{\algorithmicindent}\textbf{Input:} \\
 \hspace*{\algorithmicindent} $\: a$: The target attribute value\\
 \hspace*{\algorithmicindent} $\: V$: Vocabulary\\
 \hspace*{\algorithmicindent} $\: B > 0$: Beam size\\
 \hspace*{\algorithmicindent} $\: L > 0$: Maximum output length\\
 \hspace*{\algorithmicindent} $\: k > 0$: Number of continuations to score for each hypothesis.\\
 \hspace*{\algorithmicindent} $\: \alpha > 0$: Optional attribute weight.\\
 \hspace*{\algorithmicindent}\textbf{Output:} A string in $V*$ with length at most $L$
\begin{algorithmic}[1]
\State $X[b] = \epsilon$ for $b \in {1, \dots, B}$ \qquad\{Initialize all hypotheses to the empty sequence\}
\State $S \gets [0, -\infty, -\infty, \dots, -\infty]$ \qquad\{A length $B$ array of cumulative scores, only $S[0]$ is initially finite.\}
\State $t \gets 1$
\While{Any hypothesis $X[i]$ on the beam is not complete AND $t \le L$}
    \State Init empty $b \times k$ array $U_t$ \qquad\{Unconditional scores\}
    \State Init empty $b \times k$ array $C_t$ \qquad\{Conditional scores)\}
    \State Init empty $b \times k$ array $C'_t$ \qquad\{Weighted conditional scores, optional\}
    \State Init empty $b \times k$ array $W$ \qquad\{Continuations\}
    \For{$b = 1, \dots, B$}
        \If {$t < L$}
            \State $L[w] \gets \log\pmodel (w | x_{1:t} = X[b])$ \{for all $w \in |V|$\}
        \Else
            \State $L[:] \gets -\infty$
            \State $L[\text{\tt </s>}] \gets 0$ \qquad\{If at the max sequence length, all hypotheses are forced to be complete\}
        \EndIf
        \State $W[b, :] \gets$ words with top $k$ scores in $L$
        \For {$i = 1, \dots, k$}\qquad{}
            \State $w \gets W[b, i]$
            \State $U_t[b, i] \gets S[b] + L[w]$
            \State $C_t[b, i] \gets U[b, :] + \log\pclf(a | x_{t+1} = w, x_{1:t} = X[b])$
            \State $C'_t[b, i] \gets U[b, :] + \alpha\log\pclf(a | x_{t+1} = w, x_{1:t} = X[b])$
        \EndFor
    \EndFor
    \State \{We select new beam elements using $C'_t$, but update $S$ using $U_t$.\}
    \For{$b = 1, \dots, B$}
        \State $b_\text{prev}, i \gets$ $b$-th largest pair of indices into $C'_t$
        \State $S[b,i] \gets U_t[b_\text{prev}, i]$
        \State $X[b] \gets \mathrm{concatenate}\left(X[b_\text{prev}], W[b_\text{prev}, i]\right)$
    \EndFor
\EndWhile
\If {Attribute is deterministic}
    \State $b_\text{best} = 1$
\Else
    \State $b_\text{best} \gets \argmax\limits_{i} C_t[i]$\qquad\{If the classifier is uncertain about the value of the attribute even for a complete output, we take that into account when selecting the output.\}
\EndIf
\State \textbf{Return} $X[b_\text{best}]$
\end{algorithmic}
\end{algorithm}
