# Supplementary material for: MAP's not dead yet: Uncovering true language model modes by conditioning away degeneracy
Source: arXiv:2311.08817 source file (2024-08-08)
Supplement: Supplementary file 2 [file beam_search_derivation.tex]

\section{Derivation of conditional beam search update}

\begin{align}
    S'(x_{1:t}, a) &= \sum\limits_{i=1}^t \log P(x_i | x_{<i}, a)\\
    &= \sum\limits_{i=1}^t \log \frac{P(a | x_{\le i})P(x_i | x_{<i})}{P(a | x_{<i})}\\
    &= \left(\sum\limits_{i=1}^t \log P(x_i | x_{<i})\right) + \sum\limits_{i=1}^t \log\frac{P(a | x_{\le i})}{P(a | x_{<i})}\\
    &= S(x_{1:t}) + \log\frac{P(a | x_{\le t})}{P(a | x_{<1})}\\
    &= S(x_{1:t}) + \log\frac{P(a | x_{\le t})}{P(a )}\\
\end{align}
